# Supplementary material for: A Sampling Theorem for Deconvolution in Two Dimensions
Source: arXiv:2003.13784 source file (2020-08-04)
Supplement: Supplementary file 1 [file withheld_supplementary.tex]

We prove \Cref{lem:QBound} using \Cref{lem:Regions} by showing for large enough $\spikesep$ that $u_1$ and $u_2$ as in \Cref{lem:Regions} can be found. To accomplish this we construct radially symmetric upper bounds on $v^T\nabla^2 Qv$ and $\nabla Q^T v$ presented in \Cref{lem:Qtri} which we use for the integrals in \Cref{lem:Regions}. In this section we present a method to compute these bounds and integrals as well as arguments that simplify these computations.

\begin{comment}
Then we have that 
\begin{align}
\nabla B_1(t)\cdot\hat{t}&=\partial_xB_1(t)\cdot\frac{t_{(1)}}{\norm{t}}+\partial_yB_1(t)\cdot\frac{t_{(2)}}{\norm{t}}\\
&\leq\sup_{s^1,s^2,s^3}\partial_x B_1(t)\cdot\frac{t_{(1)}}{\norm{t}}+
%\sup_{s^1,s^2,s^3}
\partial_y B_1(t)\cdot\frac{t_{(2)}}{\norm{t}}\\
&\leq \Dt(\norm{t};\gridsep)
\end{align}
where $\hat t=t/\norm{t}$ is the unit vector in the direction of $t$.
\end{comment}
%Sections and pieces that have been moved elsewhere and edited are left here for posterity

BELOW IS COPIED INTO \Cref{sec:Envelopes}

We construct envelope functions for the bumps and waves' largest eigenvalues just as we did for the functions and their derivatives. First we derive a form for the contribution from each of the three Gaussian terms in a bump or wave. The Hessian of $f(x) = e^{-\norm{x}^2/2}$ is:
\begin{equation}
\nabla^2 f(x)=\begin{bmatrix}
(x_1^2-1)&x_1x_2\\
x_1x_2&(x_2^2-1)
\end{bmatrix}\cdot e^{-\norm{x}^2/2},
\end{equation}
so the eigenvalues are $\lambda e^{-\norm{x}^2/2}$ such that
\begin{equation}
\begin{aligned}
0&=(x_1^2-1-\lambda)(x_2^2-1-\lambda)-x_1^2x_2^2\\
%&=x_1^2x_2^2-x_1^2-\lambda x_1^2-x_2^2+1+\lambda-\lambda x_2^2+\lambda+\lambda^2-x_1^2x_2^2\\
%&=\lambda^2+2\lambda-\lambda(x_1^2+x_2^2)+1-(x_1^2+x_2^2)\\
&=\lambda^2+\lambda(2-\norm{x}^2)+(1-\norm{x}^2).
\end{aligned}
\end{equation}
Consequently,
\begin{equation}
%\lambda&=\frac{-2+\norm{x}^2\pm\sqrt{4-4\norm{x}^2+\norm{x}^4-4+4\norm{x}^2}}{2}\\
%&=\frac{-2+\norm{x}^2\pm\norm{x}^2}{2}=\norm{x}^2-1,-1
\lambda=\norm{x}^2-1,-1.
\end{equation}
If $g(x)=\kappa f(x)$ then the largest eigenvalue of $\nabla^2 g$ is
\begin{equation}\label{eq:eigenvalue}
\lambda^g_{\max}(x)=\max(\kappa(\norm{x}^2-1), -\kappa)e^{-\norm{x}^2/2}.
\end{equation}
Since every bump and wave is a sum of three Gaussians \eqref{eq:BWdefs}, their largest eigenvalue at any point is less than the sum of the largest eigenvalues from each Gaussian. For bump $B_1$ where $Q(t_1)=1$ this is
\begin{equation}
\begin{aligned}\label{eq:lmaxbBound}
\lmaxb{1}(t)&\leq
\bcone_1(\norm{s^1_1-t}^2-1)e^{-\norm{s^1_1-t}^2/2}+\bctwo_1(\norm{s^2_1-t}^2-1)e^{-\norm{s^2_1-t}^2/2}\\
&\qquad+\bcthree_1(\norm{s^3_1-t}^2-1)e^{-\norm{s^3_1-t}^2/2}.
\end{aligned}
\end{equation}
%where the samples $s^i_j$ are the centers of the Gaussians.
The following bound holds for all bumps $B_j$:
%\bdb{can they be negative? It seems more that the bump can have a negative weight on it} \jpm{Revised this to specify eigenvalue for bump at $t_1$ versus other spikes}
\begin{equation}
\begin{aligned}\label{eq:lmaxbBoundAbs}
\abs{\lmaxb{j}(t)}&\leq\abs{\bcone_j}\max(\norm{s^1_j-t}^2-1,1)e^{-\norm{s^1_j-t}^2/2}\\
&\qquad+\abs{\bctwo_j}\max(\norm{s^2_j-t}^2-1,1)e^{-\norm{s^2_j-t}^2/2}\\
&\qquad+\abs{\bcthree_j}\max(\norm{s^3_j-t}^2-1,1)e^{-\norm{s^3_j-t}^2/2}.
\end{aligned}
\end{equation}
A similar bound holds for both waves, where the value of each term depends on the associated coefficient's sign:
\begin{equation}
\begin{aligned}
\abs{\lmaxwo{j}(t)}&\leq
%\left|\max(\wocone_j(\norm{s^1_j-t}^2-1),-\wocone_j)e^{-\norm{s^1_j-t}^2/2}\right.\\
\abs{\wocone_j}\max(\norm{s^1_j-t}^2-1,1)e^{-\norm{s^1_j-t}^2/2}\\
%&\qquad+\max(\woctwo_j(\norm{s^2_j-t}^2-1),-\woctwo_j)e^{-\norm{s^2_j-t}^2/2}\\
&\qquad+\abs{\woctwo_j}\max(\norm{s^2_j-t}^2-1,1)e^{-\norm{s^2_j-t}^2/2}\\
%&\qquad\left.+\max(\wocthree_j(\norm{s^3_j-t}^2-1),-\wocthree_j)e^{-\norm{s^3_j-t}^2/2}\right|.
&\qquad+\abs{\wocthree_j}\max(\norm{s^3_j-t}^2-1,1)e^{-\norm{s^3_j-t}^2/2}.
\end{aligned}
\end{equation}
Also note that by \eqref{eq:coeffmat} one of $\woctwo_j$ and $\wocthree_j$ will be zero and similarly for $\wtctwo_j$ and $\wtcthree_j$.

As mentioned, we construct envelopes that bound $\lmaxb{j}$, $\abs{\lmaxb{j}}$,
$\abs{\lmaxwo{j}}$ and $\abs{\lmaxwt{j}}$.
$\lmaxb{j}$ will be negative at its spike $t_j$ and decay away from it. Since we want to measure the bump eigenvalue's negativity around $t_j$ this envelope should not be monotonized.
Thus the envelope is constructed by taking the supremum over points at the same distance from $t_j$ and over all positions of $t_j$ with respect to its three nearest samples $s^1_j$, $s^2_j$ and $s^3_j$:
\begin{equation}\label{eq:EVnonmon}
%\ltmaxb(r):=\sup_{\substack{{t_j,s^1_j,s^2_j,s^3_j}\\ \norm{x-t_j}=r}}\lmaxb{j}(x).
\ltmaxb(r):=\sup_{\substack{\norm{t-t_j}=r\\ s_j^1,s_j^2,s_j^3\mbox{ nearest }t_j}}\lmaxb{j}(t;t_j,s^1_j,s^2_j,s^3_j)
\end{equation}
$\ltamaxb$, $\ltmaxwo$ and $\ltmaxwt$ are monotonized by taking the supremum over $\norm{t-t_0}\geq r$ like the previous function envelopes:
\begin{equation}\label{eq:EVmon}
\begin{aligned}
\ltamaxb(r)&:=\sup_{\substack{\norm{t-t_j}\geq r\\ s_j^1,s_j^2,s_j^3\mbox{ nearest }t_j}}\abs{\lmaxb{j}(t)}\\
\ltmaxwo(r)&:=\sup_{\substack{\norm{t-t_j}\geq r\\ s_j^1,s_j^2,s_j^3\mbox{ nearest }t_j}}\abs{\lmaxwo{j}(t)}\\
\ltmaxwt(r)&:=\sup_{\substack{\norm{t-t_j}\geq r\\ s_j^1,s_j^2,s_j^3\mbox{ nearest }t_j}}\abs{\lmaxwt{j}(t)}
\end{aligned}
\end{equation}

BELOW IS COPIED INTO \Cref{sec:DDQ}

By considering the largest eigenvalue of each bump and wave's Hessian, for $t_0$ such that $Q(t_0)=1$ the quantity in the integrand of \eqref{eq:Integral1} is less than the following sum at any point $t$:
\begin{equation}
\begin{aligned}
v^T\nabla^2Q(t)v&=\ \sum_{j=0} v^T(\bcoeff_jH^{B_j}+\wocoeff_jH^{W^1_j}+\wtcoeff_jH^{W^2_j})\ v\\
&\leq\ll(\norm{t-t_0})+\norminf{\wocoeff}\ltmaxwo(\norm{t-t_0})+\norminf{\wtcoeff}\ltmaxwt(\norm{t-t_0})\\
&\qquad+\sum_{j=1}\norminf{\bcoeff}\ltamaxb(\norm{t-t_j})+\norminf{\wocoeff}\ltmaxwo(\norm{t-t_j})+\norminf{\wtcoeff}\ltmaxwt(\norm{t-t_j}),\label{eq:Hbound}
\end{aligned}
\end{equation}
where we define
\begin{equation}
\ll(\norm{t-t_0}):=\max(\bcoeffmin\ltmaxb(\norm{t-t_0}),\norminf{\bcoeff}\ltmaxb(\norm{t-t_0})).
\end{equation}
Recall $\bcoeffmin$ represents the smallest magnitude that $\bcoeff_0$ can be, so that $\bcoeff_0 v^T H^{B_0}v\leq\bcoeffmin\ltmaxb$ for $\ltmaxb<0$. When $\ltmaxb\geq 0$, $\bcoeff_0v^T H^{B_0}v\leq \norminf{\bcoeff}\ltmaxb$.
If \eqref{eq:Hbound} is negative for all $v$ at $t_0$, $Q$ is negative definite.
We use $\ll$ since the integrand in \eqref{eq:DDQIntegral} may rise above 0 while the integral is still negative.

If instead $Q(t_0)=-1$, a similar lower bound holds as we show $Q$ to be positive definite and swap signs and maximum eigenvalues for minimums accordingly. For both cases this shows $Q$ bends towards 0 around spikes when $\spikesep$ is sufficiently large.

\subsubsection{Constructing Eigenvalue Envelopes}\label{sec:ConstructingEigenvalueEnvelopes}

We compute envelope upper bounds on bump and wave eigenvalues for each of the supremums in \eqref{eq:EVnonmon} and \eqref{eq:EVmon} using the same methods as described in \Cref{sec:Envelopes}. As before we partition the parameters for $\gridsep$, positional argument $t$ and spike offset $u$ into intervals $I_\gridsep$, $I_t$ and $I_u$. Recall $I_t$ and $I_u$ both are intervals in $\RR^2$ or rectangles. For the bump we use the previous choices of intervals, but since the waves' coefficient signs will affect the largest wave eigenvalues we extend the range of $I_u$ to ensure all sign combinations for the coefficients of $W^1$ and $W^2$ are considered:
\begin{equation}
I_u(j,k)=[(j-1)\gridsep/40, j\gridsep/40]\times [(k-1)\gridsep/40, k\gridsep/40],\ -19\leq j,k\leq 20, 
\end{equation}
We compute upper bounds with Interval Arithmetic for the bump for all interval choices,
\begin{equation}
\wt{\ltmaxb}(k_1,k_2,k_3,k_4,k_5)\geq \sup_{\substack{\gridsep\in I_\gridsep(k_1)\\
t\in I_t(k_2,k_3)\\ s_j^1\in I_u(k_4,k_5)}} \lmaxb{j}(t;0,s_j^1,s_j^2,s_j^3),
\end{equation}
and then compute a non-monotonic envelope upper bound for $\ltmaxb(r)$ for $r\leq 10$ and for a fixed value of $\gridsep\in I_\gridsep(k_1)$ as follows:
\begin{equation}
\ltmaxb(r)
\leq\max_{k_2,k_3,k_4,k_5}\max(\wt{\ltmaxb}(k_1,k_2,k_3,k_4,k_5),10^{-10}),
\end{equation}
where $k_2$, $k_3$ range over all values where $I_t(k_2,k_3)$ contains a point $t$ with $\|t\|=r$, and $k_4$, $k_5$ take all possible values. Non-monotonicity is important here as we want to measure the negative definiteness of bump $B_0$ at the origin spike $t_0$. For other bumps a monotonic bound for $\ltamaxb$ is obtained from
\begin{gather}
\wt{\ltamaxb}(k_1,k_2,k_3,k_4,k_5)\geq \sup_{\substack{\gridsep\in I_\gridsep(k_1)\\
t\in I_t(k_2,k_3)\\ s_j^1\in I_u(k_4,k_5)}} \abs{\lmaxb{j}(t;0,s_j^1,s_j^2,s_j^3)},\\
\ltamaxb(r)
\leq\max_{k_2,k_3,k_4,k_5}\max(\wt{\ltamaxb}(k_1,k_2,k_3,k_4,k_5),10^{-10})
\end{gather}
where as before $k_2$, $k_3$ range over values where $I_t(k_2,k_3)$ contains a point $t$ such that $\norm{t}\geq r$ and $k_4,\ k_5$ take all possible values. The same is done for wave envelopes $\ltmaxwo$ and $\ltmaxwt$ using the extended range of $I_u$ for $k_4$ and $k_5$.

\subsubsection{DIVIDER}

BELOW IS REMOVED FROM \Cref{sec:QtriProof}

In order to find $u_1$, or the largest $r$ such that the first integral in \Cref{lem:Regions}
\begin{equation}\label{eq:Integral1}
\int_{0}^{r}(v^T\nabla^2Q(t_1+sv)v)(r-s)\, ds
\end{equation}
is negative about a spike $t_1$ where $Q(t_1)=1$, we construct using eigenvalues the bound \eqref{eq:RawEigBound} on the quantity $v^T\nabla^2 Qv$ that we can compute and replace in the integrand. %This approach requires a number of steps.
First we show that $v^T\nabla^2 Qv$ can be bounded by a sum of eigenvalues of the Hessians of bumps and waves in $Q$, and construct radially symmetric envelopes of these eigenvalues.
These envelopes are similar to the bump and wave envelopes described in \Cref{sec:Envelopes} and are computed using Interval Arithmetic.
Then by applying the hexagonal partition of $\RR^2$ from \Cref{sec:Geometry} we obtain a bound that holds uniformly for all spike configurations satisfying a fixed minimum separation $\spikesep$.
Next, using the partition we show the contributions from all bumps and waves beyond 10 (in units of $\sigma$) are less than marginal amounts $\epsbump$ and $\epswave$, reducing our bound to a finite sum.
We then present a rotational invariance argument that reduces our problem to showing $\int_{0}^{r}(v^T\nabla^2 Q(t_1+sv)v)(r-s)\, ds<0$ for a single direction $v$ or just points along the horizontal axis as opposed to all directions.
This makes the task less costly computationally.
Finally we describe our computational steps involving partitioning the segment and computing the integral over each sub-segment until it becomes positive which determines our limit $r$.

\subsubsection{Eigenvalue Envelopes}

%We derive a bound on $\nabla^2 Q$'s largest eigenvalue to bound $v^T\nabla^2Qv$.
Because $\nabla^2Q$ is symmetric $v^T\nabla^2 Q v$ is at most $\lambda_{\max}$. $Q$ is a sum of many terms, so its Hessian $\nabla^2Q$ is a sum of the Hessians of these terms. Let $\nabla^2B_j$ and $\lmax^{B_j}$ denote the Hessian of the $j$th bump and its largest eigenvalue respectively, and let the same be for $\nabla^2 W^1_j$ and $\lmax^{W^1_j}$ for wave $W^1_j$ and likewise for $W^2_j$. Then for any unit vector $v$,
\begin{equation}\label{eq:RayleighBound}
v^T\nabla^2Q(t)v=\ \sum_{j=1} v^T(\bcoeff_j\nabla^2 B_j+\wocoeff_j \nabla^2 W^1_j+\wtcoeff_j \nabla^2 W^2_j)\ v.
%\leq\ \sum_{j=1}\bcoeff_j\lmaxb{j}+\wocoeff_j\lmaxwo{j}+\wtcoeff_j\lmaxwt{j}.
\end{equation}
By decomposing $\nabla^2 Q$ into a sum of the Hessians of every bump and wave and using their individual eigenvalues, we can obtain a bound on $v^T\nabla^2Qv$ to use in its place in \eqref{eq:Integral1}. For it to be negative near spike $t_1$ the dominating term $\lmaxb{1}$ in \eqref{eq:RayleighBound} must be negative and large enough to offset contributions from $W^1_1$ and $W^2_1$ and the other bumps and waves.

\subsubsection{Partition into $\{U_i\}$ and Tail Bounds}

The bound \eqref{eq:Hbound} depends on the configuration of spikes $t_j$ though we require a bound that is uniform across configurations (satisfying a fixed minimum separation $\spikesep$). To obtain such, we partition $\RR^2$ into a collection of sets $\{U_j\}$ as before. If $\diam(U_j)\leq\spikesep$
then each set contains at most one spike, which we denote by $t_j$ for convenience.

Since $\ltamaxb$, $\ltmaxwo$ and $\ltmaxwt$ are all
monotonically decreasing and $d(t,U_j)\leq\norm{t-t_j}$, we get from \eqref{eq:Hbound}
\begin{equation}\label{eq:Hbound1_OLD}
\begin{aligned}
\qform{(t)}&\leq\ll(\norm{t-t_0})+\norminf{\wocoeff}\ltmaxwo(\norm{t-t_0})+\norminf{\wtcoeff}\ltmaxwt(\norm{t-t_0})\\
&\qquad+\sum_{j=2}\norminf{\bcoeff}\ltamaxb(d(t,U_j))
+\norminf{\wocoeff}\ltmaxwo(d(t,U_j))+\norminf{\wtcoeff}\ltmaxwt(d(t,U_j)).
\end{aligned}
\end{equation}
This sum is independent of configuration so it will hold for all spike configurations satisfying a minimum separation of $\diam(U_i)=\spikesep$.
The next lemma helps bound the contributions from distant bumps and waves making \eqref{eq:Hbound1_OLD} a finite sum:
\begin{lemma}\label{lem:EVTail_OLD}
If $\norm{t}\geq10$ and $\sampleprox\leq4$,
then $\abs{\lmaxb{j}(t)}$ is bounded by 
\begin{equation}\label{eq:BumpEVbound_OLD}
f(t)=6\|t\|^2\exp\left(-\frac{\|t\|^2}{2}+\sampleprox\|t\|\right)
\end{equation}
and $\abs{\lmax^{W^1_j}(t)}$ and $\abs{\lmax^{W^2_j}(t)}$ by 
\begin{equation}
f(t)=\frac{6\|t\|^2}{\gridsep}\exp\left(-\frac{\|t\|^2}{2}+\sampleprox\|t\|\right).
\end{equation}
Consequently,
\begin{equation}\label{eq:Hbound2_OLD}
\begin{aligned}
\qform{(t)}&\leq\ll(\norm{t-t_0})+\norminf{\wocoeff}\ltmaxwo(\norm{t-t_0})+\norminf{\wtcoeff}\ltmaxwt(\norm{t-t_0})\\
&\qquad+\sum_{j=1}^{N_8}\norminf{\bcoeff}\ltamaxb(d(t,U_j))
+\norminf{\wocoeff}\ltmaxwo(d(t,U_j))+\norminf{\wtcoeff}\ltmaxwt(d(t,U_j))\\
&\qquad+\norminf{\bcoeff}\epsbump+\norminf{\wocoeff}\epswave+\norminf{\wtcoeff}\epswave,
\end{aligned}
\end{equation}
where $N_8$ denotes the number of cells $U_i$ in the first eight layers.
\end{lemma}
\begin{proof}
Consider the first term in \eqref{eq:lmaxbBoundAbs}, $|\bcone_j|\max(\|s^1_j-t\|^2-1,1)e^{-\norm{s^1_j-t}^2/2}$.
%The coefficients for bump components $\bcone$, $\bctwo$ and
%$\bcthree$ are all non-negative by \Cref{lem:crossprod} ensuring there
% is no cancellation. If we define
%\begin{equation}
%\begin{aligned}
%\lb(t;t_j,s^1_j,s^2_j,s^3_j)&:=
%\bcone_j(\norm{s^1_j-t}^2-1)e^{-\norm{s^1_j-t}^2/2}+\bctwo_j(\norm{s^2_j-t}^2-1)e^{-\norm{s^2_j-t}^2/2}\\
%&\qquad+\bcthree_j(\norm{s^3_j-t}^2-1)e^{-\norm{s^3_j-t}^2/2},
%\end{aligned}
%\end{equation}
%then $\lmaxb{j}(t)\leq\lb(t;t_j,s^1_j,s^2_j,s^3_j)$.
From \eqref{eq:coeffkernelbd} we get that
\begin{equation}
\abs{\bcone_j e^{-\norm{s^1_j-t}^2/2}}\leq\exp\left(-\frac{\|t\|^2}{2}+\sampleprox\|t\|\right),
\end{equation}
and \eqref{eq:aux5} gives
\begin{equation}
\max(\abs{\norm{s^1_j-t}^2-1},1)\leq 2\norm{t}^2.
\end{equation}
The same holds for the second and third summands and so \eqref{eq:BumpEVbound} holds.
We can separate the three terms of $W^1_j$ and $W^2_j$ in the same way to get a bound for $\abs{\lmaxwo{j}}$ and $\abs{\lmaxwt{j}}$ similarly using \eqref{eq:wcoeffkernelbd} and \eqref{eq:aux5}.

From there, \Cref{lem:BumpTail} can be extended so that $f$ can be the eigenvalues of either the bump or wave functions respectively. Thus the contributions to the eigenvalues from spikes beyond layer $l=9$ are less than $\norminf{\bcoeff}\epsbump$ for the bumps and $(\norminf{\wocoeff}+\norminf{\wtcoeff})\epswave$ for all waves.
\end{proof}

\subsubsection{Rotational Invariance}\label{sec:RotationalInvariance}

Our goal is to determine for a fixed minimum separation $\spikesep$ a distance $u_1$
%about a generic spike $t_0$
such that, for all $v$ with $\norm{v}=1$, ${\int_{0}^{r}v^T\nabla^2 Q(t_0+sv)v\ (r-s)\ ds<0}$ for $0<r\leq u_1$. Then $\abs{Q(t)}<1$ is guaranteed for all points within $u_1$ of a generic spike $t_0$. Computing \eqref{eq:Hbound2} over all points in a ball of radius $r$ about $t_0$ is impossible, and even simplifying the sum by partitioning the ball into multiple smaller regions will be computationally time-consuming.
However since our envelope functions are radially symmetric we have that the bounds hold for any rotation of the spike configuration. The radial symmetry of $\ltmaxb$, $\ltamaxb$, $\ltmaxwo$, and $\ltmaxwt$ means these bounds only depend on distance by the following lemma:
\begin{lemma}\label{lem:DDQrot}
Suppose the sets $U_j$ are fixed, and
\begin{align}
\begin{split}\label{eq:DDQterm}
\ll(\norm{x-t_0})+\norminf{\wocoeff}\ltmaxwo(\norm{x-t_0})+\norminf{\wtcoeff}\ltmaxwt(\norm{x-t_0})\qquad&\\
+\sum_{j=1}\norminf{\bcoeff}\ltamaxb(d(x,U_j))
+\norminf{\wocoeff}\ltmaxwo(d(x,U_j))+\norminf{\wtcoeff}\ltmaxwt(d(x,U_j))&<c
\end{split}
\end{align}
for all $x$ on the positive horizontal axis with $\norm{x-t_0}\leq r$. Then 
\begin{equation}
v^T\nabla^2 Q(y)v<c
\end{equation}
for all $y$ such that $\norm{y-t_0}\leq r$.
\end{lemma}
\begin{proof}
Let $y$ be such that $\norm{x-t_0}=\norm{y-t_0}$. If $\phi$ is the rotation of the plane such that $\phi(x)=y$, then the sets $\{\phi(U_i)\}$ satisfy $\diam(\phi(U_i))\leq\spikesep$ and $d(x,U_j)=d(y,\phi(U_j))$. Thus,
\begin{align}
\begin{split}
\qform{(y)}&\leq\ll(\norm{y-t_0})+\norminf{\wocoeff}\ltmaxwo(\norm{y-t_0})+\norminf{\wtcoeff}\ltmaxwt(\norm{y-t_0})\\
&\qquad+\sum_{j=1}\norminf{\bcoeff}\ltamaxb(d(y,\phi(U_j)))+\norminf{\wocoeff}\ltmaxwo(d(y,\phi(U_j)))\\
&\qquad\qquad+\norminf{\wtcoeff}\ltmaxwt(d(y,\phi(U_j)))
\end{split}\\
\begin{split}
&=\ll(\norm{x-t_0})+\norminf{\wocoeff}\ltmaxwo(\norm{x-t_0})+\norminf{\wtcoeff}\ltmaxwt(\norm{x-t_0})\\
&\qquad+\sum_{j=1}\norminf{\bcoeff}\ltamaxb(d(x,U_j))+\norminf{\wocoeff}\ltmaxwo(d(x,U_j))+\norminf{\wtcoeff}\ltmaxwt(d(x,U_j))\\
\end{split}\\
&<c.
\end{align}
\end{proof}
The consequence of this lemma is that we need only compute a bound on $\qform{}$ for points along one line segment. Once we have that bound, we can integrate $\int_0^r\qform{(s)}(r-s)\ ds$ over that segment and determine the largest $r$.

\subsubsection{Integrating over Line Segments}\label{sec:IntegratingOverLineSegments}

Our bound for $\qform{}$ in \eqref{eq:Hbound2} is feasible to compute for individual points $t$ after acquiring the distances $d(t,U_j)$ for $U_j$ in the first eight layers. In order to calculate the integral, we can transform \eqref{eq:Hbound2} into a bound that holds for line segments. 

If $S$ is a set, then for all $t\in S$,
\begin{equation}
\begin{aligned}
\ll&(\norm{t-t_0})+\norminf{\wocoeff}\ltmaxwo(\norm{t-t_0})+\norminf{\wtcoeff}\ltmaxwt(\norm{t-t_0})\\
+\sum_{j=1}^{N_8}&\norminf{\bcoeff}\ltamaxb(d(t,U_j))
+\norminf{\wocoeff}\ltmaxwo(d(t,U_j))+\norminf{\wtcoeff}\ltmaxwt(d(t,U_j))\\
\quad\leq\ &\max_{t^\ast\in S}\ll (\norm{t^\ast-t_0})+\norminf{\wocoeff}\ltmaxwo(d(t_0,S))+\norminf{\wtcoeff}\ltmaxwt(d(t_0,S))\\
&+\sum_{j=1}^{N_8}\norminf{\bcoeff}\ltamaxb(d(S,U_j))
+\norminf{\wocoeff}\ltmaxwo(d(S,U_j))+\norminf{\wtcoeff}\ltmaxwt(d(S,U_j)),\\
\end{aligned}
\end{equation}
since the envelope functions $\ltamaxb$, $\ltmaxwo$ and $\ltmaxwt$ are monotonically decreasing. When $S$ is a line segment we can calculate the values $d(t_0,S)$ and $d(S,U_j)$ using the optimization software CVX \cite{CVX}. Since our envelopes are step functions the quantity $\max_{t^\ast\in S}\ll(\norm{t^\ast-t_0})$ is easy to determine. Thus for all $t\in S$,
\begin{equation}\label{eq:Hbound3}
\begin{aligned}
\qform{(t)}&\leq\max_{t^\ast\in S}\ll (\norm{t^\ast-t_0})+\norminf{\wocoeff}\ltmaxwo(d(t_0,S))+\norminf{\wtcoeff}\ltmaxwt(d(t_0,S))\\
&\qquad+\sum_{j=1}^{N_8}\norminf{\bcoeff}\ltamaxb(d(S,U_j))
+\norminf{\wocoeff}\ltmaxwo(d(S,U_j))+\norminf{\wtcoeff}\ltmaxwt(d(S,U_j))\\
&\qquad+\norminf{\bcoeff}\epsbump+\norminf{\wocoeff}\epswave+\norminf{\wtcoeff}\epswave.
\end{aligned}
\end{equation}
Using this approach to bound $\qform{(t)}$ we get the following lemma.
\begin{lemma}\label{lem:DDQRecovery}
If $u_1$ is the entry for a choice of spike separation and grid spacing $(\spikesep,\gridsep)$ in \Cref{tab:DDQTable}, we have that 
\begin{equation}\label{eq:DDQIntegral}
\int_{0}^{r}v^T\nabla^2 Q(t_0+sv)v\ (r-s)\ ds<0
\end{equation}
for all $r\in(0,u_1]$ and any unit vector $v$.
If $Q(t)>-1$, then $\abs{Q(t)}<1$ for $\norm{t}\leq u_1$.
\end{lemma}
\begin{proof}
To determine a value for $u_1$ for each choice of $\spikesep$ and $k_1$ (containing ranges for $\gridsep$), we assume $t_0$ sits at the origin and compute a bound on the integral \eqref{eq:DDQIntegral} using \eqref{eq:Hbound3} in place of $v^T\nabla^2 Qv$ over the line segment along the positive horizontal axis from $x=0$ to $\spikesep/2$.
We calculate this integral by dividing the segment into sub-segments $S_i$ for $i=1$ to $50$.
For each sub-segment we use CVX \cite{CVX} to determine $d(S_i,U_j)$ the minimum distance between $S_i$ and $U_j$ for every $U_j$ in the first eight layers of our partition, and $d(t_0,S_i)$ is the left endpoint of $S_i$.
These values are used in \eqref{eq:Hbound3} and depicted in \Cref{fig:intervalcelldists}.
The eigenvalue envelopes $\ltmaxb$, $\ltamaxb$, $\ltmaxwo$, and $\ltmaxwt$ are computed as step-functions for each $k_1$ with the same method that the bump and wave envelopes are, out to a distance $\norm{t}_2=10$ after which the envelopes are less than $2\cdot 10^{-9}$.
Then $\max_{t^\ast\in S}\ll (\norm{t^\ast-t_0})$ is just the maximum over the values the step-function envelope takes between the two endpoints of $S_i$.
The coefficients $\bcoeffmin$, $\norminf{\bcoeff}$, $\norminf{\wocoeff}$ and $\norminf{\wtcoeff}$ were previously obtained for the parameter choices and are used again here.
Thus each value in the sum can be calculated from the step-functions for each $S_i$.

% \begin{figure}[t]
%     \centering
%     \includegraphics{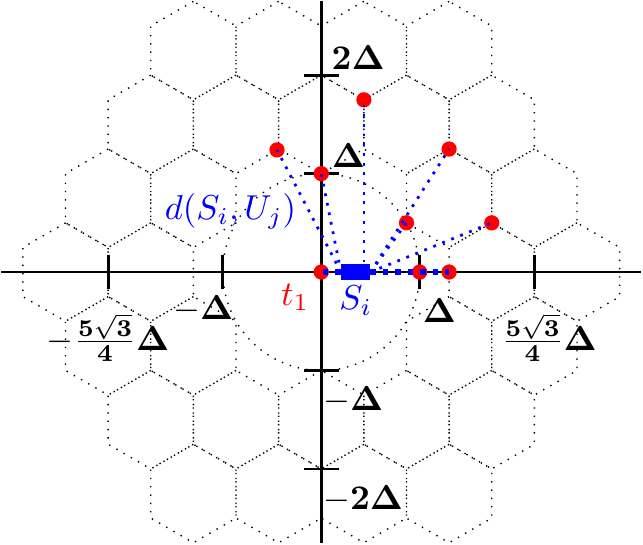}
%     \caption{Distances $d(S_i,U_j)$ depicted by lengths of blue dotted lines between red spikes in $U_j$ and blue interval $S_i$.}
%     \label{fig:intervalcelldists}
% \end{figure}

For large enough $\spikesep$ the integral from 0 through the first several $S_i$ will be negative, ensuring that $\nabla^2 Q$ is negative definite and thus $\abs{Q(t)}<1$ except at $t_0$. The endpoint of the last consecutive segment for which the integral is negative is saved as $u_1$ in \Cref{tab:DDQTable} given in units of $\spikesep$. Thus $Q(t)<1$ for all $t$ such that $\norm{t-t_0}\leq u_1$. Note it is possible that one could get better results by taking finer partitions of the line segment.
\end{proof}

\begin{sidewaystable}
\centering
\pgfplotstableread{asy/dat/Deltas.dat}\dataDeltas
\pgfplotstableread{asy/dat/DDQ.dat}\dataQ
\pgfplotstablecreatecol[copy column from table={\dataDeltas}{[index] 0}]{deltas}{\dataQ}
\pgfplotstabletypeset[fixed,
every head row/.style={before row=\hline, after row=\hline},
every last row/.style={after row=\hline},
columns={deltas,0,1,2,3,4,5,6,7,8,9,10,11,12,13,14,15},
columns/deltas/.style={column type = c|, column name=$\spikesep\backslash\gridsep$},
columns/0/.style={column name={\rotatebox{90}{$[.1,.15]$}}},
columns/1/.style={column name={\rotatebox{90}{$[.15,.2]$}}},
columns/2/.style={column name={\rotatebox{90}{$[.2,.25]$}}},
columns/3/.style={column name={\rotatebox{90}{$[.25,.3]$}}},
columns/4/.style={column name={\rotatebox{90}{$[.3,.35]$}}},
columns/5/.style={column name={\rotatebox{90}{$[.35,.4]$}}},
columns/6/.style={column name={\rotatebox{90}{$[.4,.45]$}}},
columns/7/.style={column name={\rotatebox{90}{$[.45,.5]$}}},
columns/8/.style={column name={\rotatebox{90}{$[.5,.55]$}}},
columns/9/.style={column name={\rotatebox{90}{$[.55,.6]$}}},
columns/10/.style={column name={\rotatebox{90}{$[.6,.65]$}}},
columns/11/.style={column name={\rotatebox{90}{$[.65,.7]$}}},
columns/12/.style={column name={\rotatebox{90}{$[.7,.75]$}}},
columns/13/.style={column name={\rotatebox{90}{$[.75,.8]$}}},
columns/14/.style={column name={\rotatebox{90}{$[.8,.85]$}}},
columns/15/.style={column name={\rotatebox{90}{$[.85,.89]$}}},
every odd column/.style={string replace={0.}{}},
every even column/.style={string replace={0.}{}},
empty cells with={--}
]{\dataQ}
\caption[Second Derivative Calculations]{\label{tab:DDQTable}
%\bdb{Need a clearer explanation of what the entries of the table mean.}
Entries in the table specify values for $u_1$ so that \eqref{eq:DDQIntegral} holds for $r\in(0,u_1]$.
The columns designate an interval range for $\gridsep$, and the minimum spike separation for each row is given by the left column.
$\spikesep$ and $\gridsep$ are scaled in terms of the kernel's parameter $\sigma$.
The table's entries are given in units of $\spikesep$.
Missing entries indicate that $\nabla^2 Q$ cannot be guaranteed negative definite at $t_0$ for those parameter choices and so \eqref{eq:DDQIntegral} may not hold.}
\end{sidewaystable}

%\subsection{$\nabla Q\cdot v$}\label{sec:DQ}
\subsection{\Cref{eq:RawGradBound}}

In the same manner we devise a similar bound for the term $\nabla Q(t_0+sv)\cdot v$ in the second integral of \Cref{lem:Regions} to show
\begin{equation}\label{eq:Integral2}
\int_{u_1}^{r}\nabla Q(t_0+sv)\cdot v\ ds<0,
\end{equation}
for $u_1\leq r\leq u_2$ when $Q(t_0)=1$.
Then if $Q(t)>-1$, $\abs{Q}<1$ for  $t$ with $\norm{t-t_0}\leq u_2$.
%for $T$ with sufficiently large minimum separation
%up to a distance where we can directly bound $Q$ itself.

Recall the assumption that $t_0$ is the origin and $Q(t_0)$. Like the Hessian, the directional derivative $\nabla Q(sv)\cdot v$ is a sum comprised of many terms involving the gradients of the bumps and waves for all spikes in the configuration:
\begin{equation}\label{eq:DirectionalDeriv}
\nabla Q(sv)\cdot v=\sum_{t_j\in T}\nabla [\bcoeff_jB_j(sv) + \wocoeff_jW^1_j(sv) + \wtcoeff_jW^2_j(sv)] \cdot v.
\end{equation}
And similarly the gradient of the bump at $t_0$, $\nabla B_0(t)$, is the only term in this sum that may reliably contribute a negative value for every point a distance $r$ from $t_0$. Depending on factors specific to particular configurations, the waves at $t_0$ and the terms from the other spikes might increase $\nabla Q(t)$ in the direction of $v$ depending on their location. Our method to bound the integral \eqref{eq:Integral2} involves constructing an envelope function dominating this negative term while bounding the sizes of the other terms that offset the negative part.

\subsubsection{Rotational Invariance and Integrating Over Line Segments}

Recall here we consider $t$ where $u_1\leq\norm{t-t_0}\leq\spikesep/2$.
We bound the contribution from terms in \eqref{eq:DirectionalDeriv} besides $B_0$ using the envelopes defined in \eqref{eq:Envelopes},
and if $t_j\in U_j$
%and $\diam(U_j)\leq\spikesep$ for all $j$
then $\norm{t-t_j}\geq \inf_{u\in U_j}\norm{t-u}\allowbreak=d(t,U_j)$.
%\bdb{has it been made clear why this inequality on $t$ should hold?  i.e, the assumption on the range of $\|t\|$-values we are considering should be restated in this subsection somewhere. }
Then $\nabla Q(t)\cdot \hat{t}$ can be bounded in a way that holds for all configurations with minimum separation at least $\spikesep$:
\begin{align}
\nabla Q(t)\cdot \hat{t}&=\sum_{j=0}\nabla [\bcoeff_j B_j(t)+\wocoeff_j W^1_j(t)+\wtcoeff_j W^2_j(t)]\cdot\hat{t}\\
\begin{split}
&\leq\bcoeff_0\nabla B_0(t)\cdot\hat{t}+\norminf{\wocoeff}\norm{\nabla W^1_0(t)}+\norminf{\wtcoeff}\norm{\nabla W^2_0(t)}\\
&\qquad+\sum_{j=1}\norminf{\bcoeff}\norm{\nabla B_j(t)}+\norminf{\wocoeff}\norm{\nabla W^1_j(t)}+\norminf{\wtcoeff}\norm{\nabla W^2_j(t)}
\end{split}\\
\begin{split}
&\leq\bcoeff_0\nabla B_0(t)\cdot\hat{t}+\norminf{\wocoeff}\norm{\nabla W^1_0(t)}+\norminf{\wtcoeff}\norm{\nabla W^2_0(t)}\\
&\qquad+\sum_{j=1}^{N_8}\norminf{\bcoeff}\norm{\nabla B_j(t)}+\norminf{\wocoeff}\norm{\nabla W^1_j(t)}+\norminf{\wtcoeff}\norm{\nabla W^2_j(t)}\\
&\qquad+2\norminf{\bcoeff}\epsbump+2\norminf{\wocoeff}\epswave+2\norminf{\wtcoeff}\epswave
\end{split}\\
\begin{split}\label{eq:Dbound1_OLD}
&\leq\DD(\norm{t})+\norminf{\wocoeff}\brac{\enva{\partial_x W^1}(\norm{t})^2+\enva{\partial_y W^1}(\norm{t})^2}^{1/2}\\
&\qquad+\norminf{\wtcoeff}\brac{\enva{\partial_x W^2}(\norm{t})^2+\enva{\partial_y W^2}(\norm{t})^2}^{1/2}\\
&\qquad+\sum_{j=1}^{N_8}\norminf{\bcoeff}\brac{\enva{\partial_x B}(\norm{t-t_j})^2+\enva{\partial_y B}(\norm{t-t_j})^2}^{1/2}\\
&\qquad\qquad+\norminf{\wocoeff}\brac{\enva{\partial_x W^1}(\norm{t-t_j})^2+\enva{\partial_y W^1}(\norm{t-t_j})^2}^{1/2}\\
&\qquad\qquad+\norminf{\wtcoeff}\brac{\enva{\partial_x W^2}(\norm{t-t_j})^2+\enva{\partial_y W^2}(\norm{t-t_j})^2}^{1/2}\\
&\qquad+2\norminf{\bcoeff}\epsbump+2\norminf{\wocoeff}\epswave+2\norminf{\wtcoeff}\epswave
\end{split}\\
\begin{split}\label{eq:Dbound2_OLD}
&\leq\DD(\norm{t})+\norminf{\wocoeff}\brac{\enva{\partial_x W^1}(\norm{t})^2+\enva{\partial_y W^1}(\norm{t})^2}^{1/2}\\
&\qquad+\norminf{\wtcoeff}\brac{\enva{\partial_x W^2}(\norm{t})^2+\enva{\partial_y W^2}(\norm{t})^2}^{1/2}\\
&\qquad+\sum_{j=1}^{N_8}\norminf{\bcoeff}\brac{\enva{\partial_x B}(d(t,U_j))^2+\enva{\partial_y B}(d(t,U_j))^2}^{1/2}\\
&\qquad\qquad+\norminf{\wocoeff}\brac{\enva{\partial_x W^1}(d(t,U_j))^2+\enva{\partial_y W^1}(d(t,U_j))^2}^{1/2}\\
&\qquad\qquad+\norminf{\wtcoeff}\brac{\enva{\partial_x W^2}(d(t,U_j))^2+\enva{\partial_y W^2}(d(t,U_j))^2}^{1/2}\\
&\qquad+2\norminf{\bcoeff}\epsbump+2\norminf{\wocoeff}\epswave+2\norminf{\wtcoeff}\epswave.
\end{split}
\end{align}
We use the next lemma to show rotational invariance and reduce the problem to showing the bound is negative on a segment:
\bdb{sum below has no upper bound.}
\begin{lemma}\label{lem:DQrot}
Suppose $t_0$ is the origin, and
\begin{equation}
\begin{gathered}
\label{eq:Dbound3}
\DD(\norm{t})+\norminf{\wocoeff}\brac{\enva{\partial_x W^1}(\norm{t})^2+\enva{\partial_y W^1}(\norm{t})^2}^{1/2}\\
+\norminf{\wtcoeff}\brac{\enva{\partial_x W^2}(\norm{t})^2+\enva{\partial_y W^2}(\norm{t})^2}^{1/2}\\
+\sum_{j=1}\norminf{\bcoeff}\brac{\enva{\partial_x B}(d(t,U_j))^2+\enva{\partial_y B}(d(t,U_j))^2}^{1/2}\\
+\norminf{\wocoeff}\brac{\enva{\partial_x W^1}(d(t,U_j))^2+\enva{\partial_y W^1}(d(t,U_j))^2}^{1/2}\\
+\norminf{\wtcoeff}\brac{\enva{\partial_x W^2}(d(t,U_j))^2+\enva{\partial_y W^2}(d(t,U_j))^2}^{1/2}\\
+2\norminf{\bcoeff}\epsbump+2\norminf{\wocoeff}\epswave+2\norminf{\wtcoeff}\epswave
\end{gathered}
\end{equation}
is negative for $t$ on the positive horizontal axis with $r_1\leq\norm{t}\leq r_2$. Then $\nabla Q(t)\cdot \hat{t}<0$ for all $t$ such that $r_1\leq\norm{t}\leq r_2$.
\end{lemma}
\begin{proof}
The proof follows the same steps as \Cref{lem:DDQrot}, that for every $t$ there exists $y$ on the horizontal axis with $\norm{y}=\norm{t}$ and a rotation $\phi$ where $\phi(t)=y$ so that $d(t,U_j)=d(y,\phi(U_j))$. If \eqref{eq:Dbound3} is negative for $y$ and $\phi(U_j)$ then $\nabla Q(t)\cdot \hat{t}$ is also negative.
\end{proof}
As before to show \eqref{eq:Integral2} we can transform \eqref{eq:Dbound3} into a bound that holds for line segments. If $S$ is a segment and $t\in S$ then $\norm{t-t_0}\geq d(t_0,S)$, $d(t,U_j)\geq d(S,U_j)$ and $\DD(\norm{t})\leq\max_{t^\ast\in S}\DD(\norm{t^\ast})$. Substituting these into \eqref{eq:Dbound3} gives a bound for $\nabla Q(t)\cdot \hat{t}$ that holds uniformly over points in $S$:
\begin{equation}
\begin{split}\label{eq:Dbound4}
\nabla Q(t)\cdot \hat{t}
&\leq\max_{t^\ast\in S}\DD(\norm{t^\ast})+\norminf{\wocoeff}\brac{\enva{\partial_x W^1}(d(t_0,S))^2+\enva{\partial_y W^1}(d(t_0,S))^2}^{1/2}\\
&\qquad+\norminf{\wtcoeff}\brac{\enva{\partial_x W^2}(d(t_0,S))^2+\enva{\partial_y W^2}(d(t_0,S))^2}^{1/2}\\
&\qquad+\sum_{j=1}^{N_8}\norminf{\bcoeff}\brac{\enva{\partial_x B}(d(S,U_j))^2+\enva{\partial_y B}(d(S,U_j))^2}^{1/2}\\
&\qquad\qquad+\norminf{\wocoeff}\brac{\enva{\partial_x W^1}(d(S,U_j))^2+\enva{\partial_y W^1}(d(S,U_j))^2}^{1/2}\\
&\qquad\qquad+\norminf{\wtcoeff}\brac{\enva{\partial_x W^2}(d(S,U_j))^2+\enva{\partial_y W^2}(d(S,U_j))^2}^{1/2}\\
&\qquad+2\norminf{\bcoeff}\epsbump+2\norminf{\wocoeff}\epswave+2\norminf{\wtcoeff}\epswave.
\end{split}
\end{equation}
Then we can prove the next lemma.
%relying on Mathematica for computations:
\begin{lemma}\label{lem:DQRecovery}
If $u_2$ is the entry in \Cref{tab:DQTable} for a choice of spike separation and grid spacing $(\spikesep,\gridsep)$, then there exists $u_1\in(0,u_2]$ such that $\abs{Q(t)}<1$ for $\norm{t}\leq u_1$ and
\begin{equation}\label{eq:DQIntegral}
%\int_{0}^{u_1}v^T\nabla^2 Q(t_0+sv)v\ (u_1-s)\ ds+
\int_{u_1}^{r}\nabla Q(t_0+sv)\cdot v\ ds<0
\end{equation}
for all $r\in(u_1,u_2]$ and $v$ with $\norm{v}=1$.
If $Q(t)>-1$, then $\abs{Q(t)}<1$ for $\norm{t}\leq u_2$.
\end{lemma}
\begin{proof}
We extend the region where we can show $\abs{Q}<1$ by computing a bound on \eqref{eq:DQIntegral} using \eqref{eq:Dbound4} in place of $\nabla Q(t_0+sv)\cdot v$
and calculating this integral on the segment along the positive horizontal axis from $x=0$ to $\spikesep/2$.
We divide this segment into sub-segments $S_i$ for $i=1$ to 50, and this integral provides an upper bound on the change in $Q$ over each $S_i$.
As per \Cref{lem:Regions}, if this integral is negative over consecutive $S_i$ that overlap $u_1$ from \Cref{tab:DDQTable}, i.e. from $i=i_1,\ldots,i_2$ where $\cup_{i=i_1}^{i_2} S_i=[a,u_2]$ with $a\leq u_1$, then $Q(t)<1$ for $t$ with $\norm{t-t_0}\leq u_2$. If $a>u_1$ the bound cannot be guaranteed.
Thus we aim to show this integral is negative on segments left of $u_1$.

The entries in \Cref{tab:DQTable} give values for $u_2$ in units of $\spikesep$ for choice of $(\spikesep,\gridsep)$ where $u_1$ exists in \Cref{tab:DDQTable} and where \eqref{eq:DQIntegral} is negative over $[a,u_2]$ for $a\leq u_1$.
$d(S_i,U_j)$ and $d(t_0,S_i)$ in \eqref{eq:Dbound4} are previously calculated from \Cref{lem:DDQRecovery}, and step-function envelopes for $\Dt$ are calculated for each $k_1$ specifying $I_\gridsep(k_1)$ containing $\gridsep$.
$\DD$ is obtained using \eqref{eq:DDdef}.
We compute this bound on \eqref{eq:DQIntegral} over each sub-segment $S_i$ and determine $[a,u_2]$ where $Q$ decreases.
Thus for $u_2$ in \Cref{tab:DQTable}, $Q(t)<1$ is guaranteed for $\norm{t}\leq u_2$.
If $Q>-1$ then $\abs{Q(t)}<1$ for such $t$.
\end{proof}

\begin{sidewaystable}
\centering
\pgfplotstableread{asy/dat/Deltas.dat}\dataDeltas
\pgfplotstableread{asy/dat/DQ.dat}\dataQ
\pgfplotstablecreatecol[copy column from table={\dataDeltas}{[index] 0}]{deltas}{\dataQ}
\pgfplotstabletypeset[fixed,
every head row/.style={before row=\hline, after row=\hline},
every last row/.style={after row=\hline},
columns={deltas,0,1,2,3,4,5,6,7,8,9,10,11,12,13,14,15},
%columns={deltas,0,1,2,3,4,5,6,7},
columns/deltas/.style={column type = c|, column name=$\spikesep\backslash\gridsep$},
columns/0/.style={column name={\rotatebox{90}{$[.1,.15]$}}},
columns/1/.style={column name={\rotatebox{90}{$[.15,.2]$}}},
columns/2/.style={column name={\rotatebox{90}{$[.2,.25]$}}},
columns/3/.style={column name={\rotatebox{90}{$[.25,.3]$}}},
columns/4/.style={column name={\rotatebox{90}{$[.3,.35]$}}},
columns/5/.style={column name={\rotatebox{90}{$[.35,.4]$}}},
columns/6/.style={column name={\rotatebox{90}{$[.4,.45]$}}},
columns/7/.style={column name={\rotatebox{90}{$[.45,.5]$}}},
columns/8/.style={column name={\rotatebox{90}{$[.5,.55]$}}},
columns/9/.style={column name={\rotatebox{90}{$[.55,.6]$}}},
columns/10/.style={column name={\rotatebox{90}{$[.6,.65]$}}},
columns/11/.style={column name={\rotatebox{90}{$[.65,.7]$}}},
columns/12/.style={column name={\rotatebox{90}{$[.7,.75]$}}},
columns/13/.style={column name={\rotatebox{90}{$[.75,.8]$}}},
columns/14/.style={column name={\rotatebox{90}{$[.8,.85]$}}},
columns/15/.style={column name={\rotatebox{90}{$[.85,.89]$}}},
% columns/0/.style={column name={$[.1,.15]$}},
% columns/1/.style={column name={$[.15,.2]$}},
% columns/2/.style={column name={$[.2,.25]$}},
% columns/3/.style={column name={$[.25,.3]$}},
% columns/4/.style={column name={$[.3,.35]$}},
% columns/5/.style={column name={$[.35,.4]$}},
% columns/6/.style={column name={$[.4,.45]$}},
% columns/7/.style={column name={$[.45,.5]$}},
every odd column/.style={string replace={0.}{}},
every even column/.style={string replace={0.}{}},
empty cells with={--}
]{\dataQ}
\caption[First Derivative Calculations]{\label{tab:DQTable} Missing entries are those for which either no $t_1$ exists such that \eqref{eq:DQIntegral} is negative, $\norminf{\bcoeff}$, $\norminf{\wocoeff}$ and $\norminf{\wtcoeff}$ could not be computed, or $v^THv>0$ at $t=0$.}
\end{sidewaystable}

\subsection{Bounding $\abs{Q}$ Directly}\label{sec:Q}

We can check directly that $\abs{Q}<1$ for $\norm{t}\geq u_2$ using the bump and wave envelope functions $\enva{B}$, $\enva{W^1}$ and $\enva{W^2}$. For $t\in S$,
\begin{align}
\abs{Q(t)}&=\abs{\sum_{j=0}\bcoeff_j B_j(t)+\wocoeff_j W^1_j(t)+\wtcoeff_j W^2_j(t)}\\
%\begin{split}
%&\leq\norminf{\bcoeff}\enva{B}(\norm{x})+\norminf{\wocoeff}\enva{W^1}(\norm{x})+\norminf{\wtcoeff}\enva{W^2}(\norm{x})\\
%&\qquad+\sum_{j=2}\norminf{\bcoeff}\enva{B}(\norm{x-t_j})+\norminf{\wocoeff}\enva{W^1}(\norm{x-t_j})+\norminf{\wtcoeff}\enva{W^2}(\norm{x-t_j})
%\end{split}\\
\begin{split}\label{eq:Qenvbound}
&\leq\norminf{\bcoeff}\enva{B}(d(t_0,S))+\norminf{\wocoeff}\enva{W^1}(d(t_0,S))+\norminf{\wtcoeff}\enva{W^2}(d(t_0,S))\\
&\qquad+\sum_{j=1}^{N_8}\norminf{\bcoeff}\enva{B}(d(S,U_j))+\norminf{\wocoeff}\enva{W^1}(d(S,U_j))+\norminf{\wtcoeff}\enva{W^2}(d(S,U_j))\\
&\qquad+\norminf{\bcoeff}\epsbump+\norminf{\wocoeff}\epswave+\norminf{\wtcoeff}\epswave.
\end{split}
\end{align}
\eqref{eq:Qenvbound} is independent of spike configuration so it holds for all configurations having minimum separation $\spikesep\geq\diam(U_j)$.
Again rotational invariance is easily shown so we need only show $\abs{Q}<1$ for $t$ on the positive horizontal axis from $u_2$ in \Cref{tab:DQTable} to $\spikesep/2$, and that $Q(t)>-1$ for $\norm{t}\leq\spikesep/2$.
The next lemma resolves \Cref{lem:QBoundNear}:
\begin{lemma}
$\abs{Q(t)}<1$ for $\norm{t}\leq\spikesep/2$ for the choices of $\spikesep$ and $\gridsep$ indicated in \Cref{fig:RecoveryMapFirst}.
\end{lemma}
\begin{proof}
First, to show $Q(t)>-1$ for each $S_i$ as required by \Cref{lem:Regions}, note that since $B_0(t)>0$,
\begin{equation}
\begin{aligned}
Q(t)&>-\norminf{\wocoeff}\enva{W^1}(d(t_0,S_i))-\norminf{\wtcoeff}\enva{W^2}(d(t_0,S_i))\\
&\qquad-\left(\sum_{j=1}^{N_8}\norminf{\bcoeff}\enva{B}(d(S_i,U_j))+\norminf{\wocoeff}\enva{W^1}(d(S_i,U_j))+\norminf{\wtcoeff}\enva{W^2}(d(S_i,U_j))\right)\\
&\qquad-\norminf{\bcoeff}\epsbump-\norminf{\wocoeff}\epswave-\norminf{\wtcoeff}\epswave.
\end{aligned}
\end{equation}
As before this sum is computed for each sub-segment $S_i$ so that the choices of $\spikesep$ and $\gridsep$ where $Q(t)>-1$ are indicated by the blue shaded region in \Cref{fig:LowerBoundMap}.

Next the sum \eqref{eq:Qenvbound} is performed for each sub-segment $S_i$ using the bump and wave envelopes. If the sum for each $S_i$ from $u_2$ to $\spikesep/2$ is bounded by 1 then \Cref{lem:Regions} is satisfied and so $\abs{Q(t)}<1$ is guaranteed for $\norm{t}\leq\spikesep/2$. The parameter choices $(\spikesep,\gridsep)$ satisfying this are shown in \Cref{fig:RecoveryMapFirst}.
Thus \Cref{lem:QBoundNear} is resolved.
\end{proof}
\begin{figure}
\centering
\includegraphics[scale=0.5]{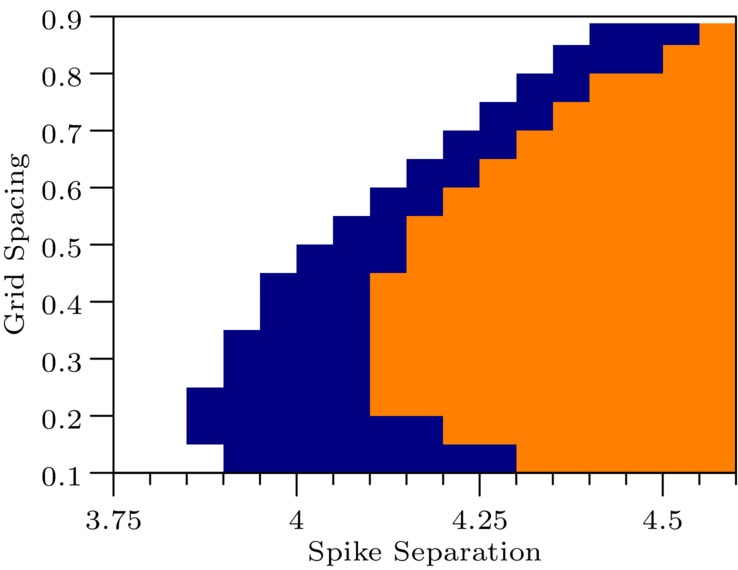}
\caption[Boundedness of $\abs{Q}$]{Recovery map in orange superimposed on regions where $Q>-1$ in dark blue.}
\label{fig:LowerBoundMap}
\end{figure}

%\begin{lemma}
%\label{lem:Qrot}
%If for $t$ on the positive horizontal axis with $r_3\leq\norm{t}\leq\spikesep/2$ 
%\begin{align}
%\begin{split}\label{eq:Qterm}
%\norminf{\bcoeff}\enva{B}(\norm{x})+\norminf{\wocoeff}\enva{W^1}(\norm{x})+\norminf{\wtcoeff}\enva{W^2}(\norm{x})&\\
%\qquad+\sum_{j=2}\norminf{\bcoeff}\enva{B}(d(x,U_j))+\norminf{\wocoeff}\enva{W^1}(d(x,U_j))+\norminf{\wtcoeff}\enva{W^2}(d(x,U_j))&<1
%\end{split}
%\end{align}
%then
%\begin{equation}
%\abs{Q}<1
%\end{equation}
%for all $x$ such that $r_3\leq\norm{x}\leq\spikesep/2$.
%\end{lemma}
